# Supplementary material for: Dynamical structure factors of Warm Dense Matter from Time-Dependent Orbital-Free and Mixed-Stochastic-Deterministic Density Functional Theory
Source: arXiv:2410.23599 ancillary file (2024-11-01)
Supplement: Supplementary file 1 [file Supp_Mat.pdf]

**Supplemental Material for**

# Dynamical structure factors of Warm Dense Matter from Time-Dependent Orbital-Free and Mixed-Stochastic-Deterministic Density Functional Theory

Alexander J. White[1]
[1] *Theoretical Division, Los Alamos National Laboratory, Los Alamos, NM 87545, USA*
(Dated: October 31, 2024)

## S1. SIMULATION DETAILS

All simulations in the letter are preformed using the pseudopotential plane-wave DFT code `SHRED` (Stochastic and Hybrid Representation of Electronic structure by Density functional theory) developed by the author at Los Alamos National Laboratory [1, 2]. Table S1 shows the parameters used to perform the simulations. All simulations use the semilocal Perdew-Burke-Ernzerhof exchange correlation functional.[3] For Kohn Sham calculations, we utilize Optimized Norm-Conserving Vanderbilt pseudopotentials [4] (ONCV, version 3.2.3) from the PseudoDojo repository [5]. For Orbital free calculations we generate local regularized pseudopotentials using the approach developed by Flavien Lambert,[6] and fit the pseudopotential to a Gaussian, Goedecker-Teter-Hutter (GTH), form for utilization in SHRED.[7]

For molecular dynamics we utilize the isokinetic ensemble starting our simulation from random ion positions, allowing for equilibration, and then sampling snapshots.

For time dependent DFT we utilize the Short Iterative Lanczos propagation scheme [8], with no enforced time reversal symmetry. The perturbing electric field is aligned along the y axis which is adjusted such that the perturbing wavevector is commiserate with the reciprocal space grid.

TABLE S1: Simulation parameters for the letter and supplemental materials. Key: $\rho$ - total mass density, $k_BT$ - electron temperature, $N_\psi$ - number of deterministic Kohn Sham orbitals, $N_\chi$ - number of complementary stochastic vectors (0 for both indicates orbital free), k-grid (x/y/z) - Broullion Zone sample via Monkhorst-Pack grids (no $\Gamma$) [9], $N_a$ - number of atoms in unit cell, Ecut - maximum planewave energy defining basis and real-space grid, $\gamma$ - the Gaussian dampening coefficient / broadening parameter for KS/TFW+D/TFW, $E_0$ - the perturbing electric field strength, $dt$ the electronic time step. $t_w$ the time width of the perturbing electric field Gaussian envelope. $t_0$ the peak time of the perturbing electric field Gaussian envelope.

| System | $\rho$ [g/cm$^3$] | $k_BT$ [eV] | $N_\psi$ | $N_\chi$ | k-grid | $N_a$ | Ecut [eV] | $\gamma$ [eV] | $E_0$[a.u.] | $dt$ [a.u.] | $t_w[a.u.]$ | $t_0[a.u.]$ |
|---|---|---|---|---|---|---|---|---|---|---|---|---|
| | | | | | –Molecular Dynamics– | | | | | | | |
| Be (KS) | 5.5 | 13 | 288 | 72 | $\Gamma$ | 64 | 1200 | N/A | N/A | 7.0 | N/A | N/A |
| Be (KS) | 1.86 | 53.0 | 168 | 28 | $\Gamma$ | 64 | 1250 | N/A | N/A | 5.0 | N/A | N/A |
| CH (1:1, KS) | 6.05 | 10.0 | 468 | 0 | $\Gamma$ | 32:32 | 1350 | N/A | N/A | 2.3 | N/A | N/A |
| Al (WDM) | 2.7 | 6.0 | 336 | 28 | $\Gamma$ | 64 | 675 | N/A | N/A | 32.6 | N/A | N/A |
| | | | | | –TD-DFT– | | | | | | | |
| Be (KS) | 5.5 | 13 | 384 | 128 | $1\times2\times1$ | 64 | 1200 | 1/1/5 | 0.1 | .018 | 0.1 | 0.5 |
| Be (KS) | 1.86 | 53.0 | 1344 | 448 | $1\times2\times1$ | 4 | 1250 | 1/1/5 | 0.1 | 0.002 | 0.1 | 0.05 |
| CH (1:1, KS) | 6.05 | 10.0 | 512 | 0 | $1\times4\times1$ | 4 | 1350 | 1/1/7 | 0.01 | 0.002 | 0.01 | 0.05 |
| Al (WDM) | 2.7 | 6.0 | 320 | 64 | $2\times4\times2$ | 32 | 675 | 0.01/0.01/2 | 0.1 | 0.032 | 0.1 | 0.5 |

[1] A. J. White and L. A. Collins, Fast and Universal Kohn-Sham Density Functional Theory Algorithm for Warm Dense Matter to Hot Dense Plasma, Phys. Rev. Lett. **125**, 055002 (2020).
[2] A. J. White, L. A. Collins, K. Nichols, and S. X. Hu, Mixed stochastic-deterministic time-dependent density functional theory: application to stopping power of warm dense carbon, Journal of Physics: Condensed Matter **34**, 174001 (2022).
[3] J. P. Perdew, K. Burke, and M. Ernzerhof, Generalized gradient approximation made simple, Phys. Rev. Lett. **77**, 3865 (1996).
[4] D. R. Hamann, Optimized norm-conserving Vanderbilt pseudopotentials, Phys. Rev. B **88**, 085117 (2013).

[5] M. van Setten, M. Giantomassi, E. Bousquet, M. Verstraete, D. Hamann, X. Gonze, and G.-M. Rignanese, The PseudoDojo: Training and grading a 85 element optimized norm-conserving pseudopotential table, Computer Physics Communications **226**, 39 (2018).
[6] F. Lambert, J. Clérouin, and G. Zérah, Very-high-temperature molecular dynamics, Phys. Rev. E **73**, 016403 (2006).
[7] S. Goedecker, M. Teter, and J. Hutter, Separable dual-space Gaussian pseudopotentials, Phys. Rev. B **54**, 1703 (1996).
[8] T. J. Park and J. C. Light, Unitary quantum time evolution by iterative Lanczos reduction, The Journal of Chemical Physics **85**, 5870 (1986).
[9] H. J. Monkhorst and J. D. Pack, Special points for Brillouin-zone integrations, Phys. Rev. B **13**, 5188 (1976).
